# Supplementary material for: Discovering Pattern Structure Using Differentiable Compositing
Source: arXiv:2010.08788 source file (2020-10-17)
Supplement: Supplementary file 1 [file 07_Supplementary.tex]

\section{Supplementary}

% \begin{algorithm}[h]
% \SetAlgoLined
% \KwResult{processed compositing parameters P}
%  $P\longleftarrow \phi $\;
%     \ForEach{$ i $}{
%         \If{$ p_i < p_{threshold} $}{
%             $ POP({\tau}_i, c_i, \theta_i, z_i) $\;
%         }
%     }
%  $\hat{\tau} = argmax(\tau)$\;
%  $\tau, c, \theta, z = Sort(\tau, c, \theta, z)\ based\ on \ z$\;
%  $P \gets P \cup (\hat{\tau}_0, c_0, \theta_0, z_0)$\;

%     \ForEach{$ i $}{
%         \eIf{$ L2(c_i, c_j) >Distance_{threshold}, \forall c_j  \in P$}{
%             $ P \gets P \cup ({\tau}_i, c_i, \theta_i, z_i)  $\;
%         }
%         {
%             \If{$ L2(c_i, c_j) <Distance_{threshold}, \forall c_j  \in P, \hat{\tau_i} \neq  \hat{\tau_j} $}{
%             $ P \gets P \cup ({\tau}_i, c_i, \theta_i, z_i) $\;
%             }
%         }
%     }
%  \caption{Continuous2Discrete(R)}
% \end{algorithm}
% I our experiments we use $p_{threshold}$ as 0.7 and $Distance_{threshold}$ as 10px for large $H_i$ and  5px for small $H_i$

% \vspace{2in}
